# Supplementary material for: Multi-resolution Guided 3D GANs for Medical Image Translation
Source: arXiv:2412.00575 source file (2024-11-30)
Supplement: Supplementary file 1 [file supplement.pdf]

# Supplementary Material

As for the supplementary materials, we submitted a zip file to enhance reproducible and present detailed information including full experiment results we could not add in the paper due to page limit. The zip file includes (1) code submission and (2) supplementary documents. Our code submission has codes for training, inferencing, evaluating, visualization, example run codes, and full quantitative results. Furthermore, we included pre-trained weights and demo data in Google Drive (see README.md in code submission for link). For documentation, below contents show the supplementary material as in text.

## 1 Implementation Details

Here are the list of implementation details such as environment settings we used:

- CPU: 2 AMD EPYC 74F3 processors
- GPU: 1 RTX A40 (takes approx. up to 40GB)
- RAM Usage: Approximately 16GB for each experiment (both train and inference)
- VRAM Usage: Approximately 35GB in training (16GB minimum required with reduced batch size) and 1.6GB in inference
- Tools used: Python, PyTorch, MONAI, and others
- Model Size (# of parameters): 6.1M for generator, 0.6M for discriminator
- Activation function: Leaky ReLU with with 0.2 negative_slope
- Pre-trained model and node used for Perception loss: VGG19 implemented in torchvision with features.35 for node
- Optimizer: Adam optimizer with learning rate of $1 \times 10^{-4}$
- Scheduler: multi-step scheduler with $t = 200$, 400, 600, 800 and $\gamma = 0.5$

Note that, for VRAM consumption, while it takes approximately 35GB VRAM for training with our hyper-parameters, inference for $586 \times 410 \times 151$ resolution image (maximum resolution across all datasets) only takes 1.6GB. This is due to patch-wise inference. This first operates model function per patch, then aggregates processed patches at last. With patch-wise processing, it only requires VRAM operations for one patch $96 \times 96 \times 96$ in resolution at a time. Note that parallel operation can be applied as well to speed up the inference (hyper-parameters we used are included in next section "Parameters used for sliding-window inferencing").

## 2 Parameters used for sliding-window inferencing

For sliding-window inferencing with Gaussian blending, we used MONAI's implementation. Here below are the exact parameter we used:

- roi_size: [96,96,96]
- overlap: 0.625
- mode: gaussian
- sigma_scale: 0.125

And here below are the code we used:

```
def sliding_window(x_input, network, patch_size=[96,96,96]):
    out = monai.inferers.sliding_window_inference(x_input, \\
            roi_size = patch_size, predictor = network, \\
            overlap = 0.625, mode = 'gaussian', \\
            sigma_scale = 0.125)
    return out
```

The exact code can be found in code submission.

## 3 Dataset Details

In addition to brief description written in the paper, we collected more information including average voxel space we used for experiments.

| Name | # of samples | Modality used | Average voxel space (in $mm^3$) |
|---|---|---|---|
| HCP1200 | 1,111 | T1, T2 MRIs | [0.7,0.7,0.7] |
| dHCP | 40 | T1, T2 MRIs | [1,1,1] |
| BraTS2021 | 1,251 | T2, Flair MRIs | [1,1,1] |
| SynthRAD ($T1\ MRI \rightarrow CT$) | 180 | T1 MRI, CT | [1,1,2.5] |
| SynthRAD ($CBCT \rightarrow CT$) | 180 | CBCT, CT | [1,1,2.5] |

For HCP1200, the exact number of patients we were able to download was 1,111. The number of patient was not exact 1,200.

## 4 Segmentation model used for brain tumor segmentation

```
model = monai.networks.nets.UNet(
    spatial_dims = 3,
    in_channels = 1,
    out_channels = 3,
    channels = [32,64,128,256,512],
    strides = [2,2,2,2],
    num_res_units=4
)
```

# 5 Organs used for TotalSegmentator

TotalSegmentator is the segmentation model for abdomen. Since this share the organs in pelvis, we used the 17 organs out of 32 possible organs that TotalSegmentator can predict since the other organs were not present in our dataset. 17 organs include: colon, urinary_bladder, sacrum, iliac_artery_right, iliac_vena_left, iliac_artery_left, iliac_vena_right, femur_left, femur_right, hip_left, hip_right, gluteus_maximus_right, gluteus_maximus_left, gluteus_medius_right, gluteus_minimus_right, iliopsoas_right, and iliopsoas_left.

# 6 Additional Sample Figures

Due to page-limit, we could not add the holistic view of the sample figures for each experiment. Here, we include them for each experiment. More visualizations can be generated using pre-trained model, visualization demo code, and sample data in code submission (weights and data should be downloaded from Google Drive from README.md).

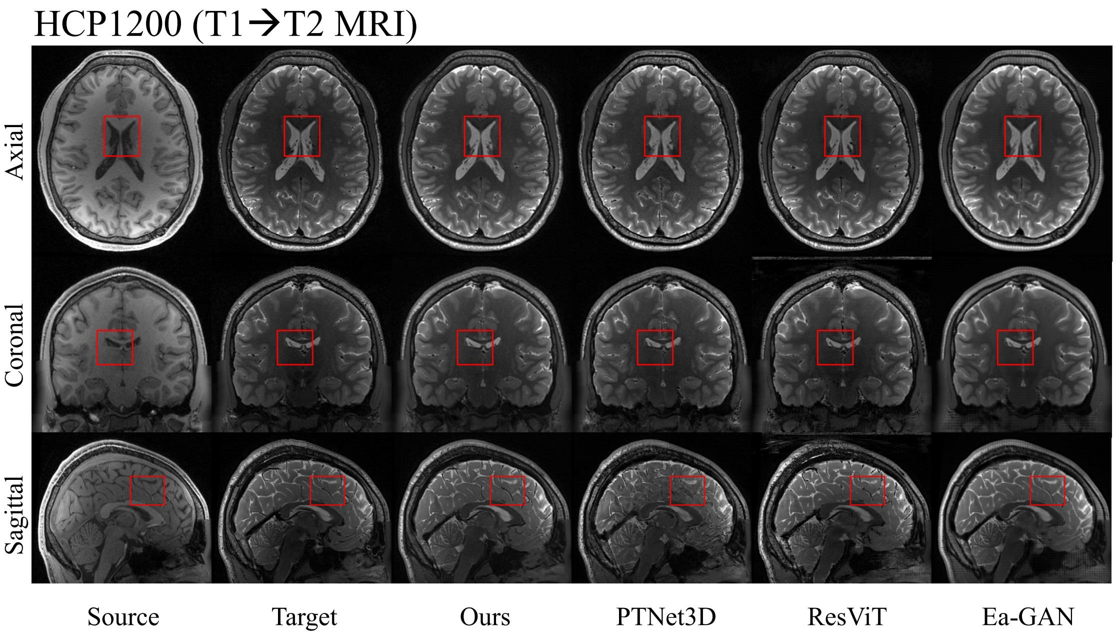
HCP1200 (T1→T2 MRI)
Axial
Coronal
Sagittal
Source
Target
Ours
PTNet3D
ResViT
Ea-GAN

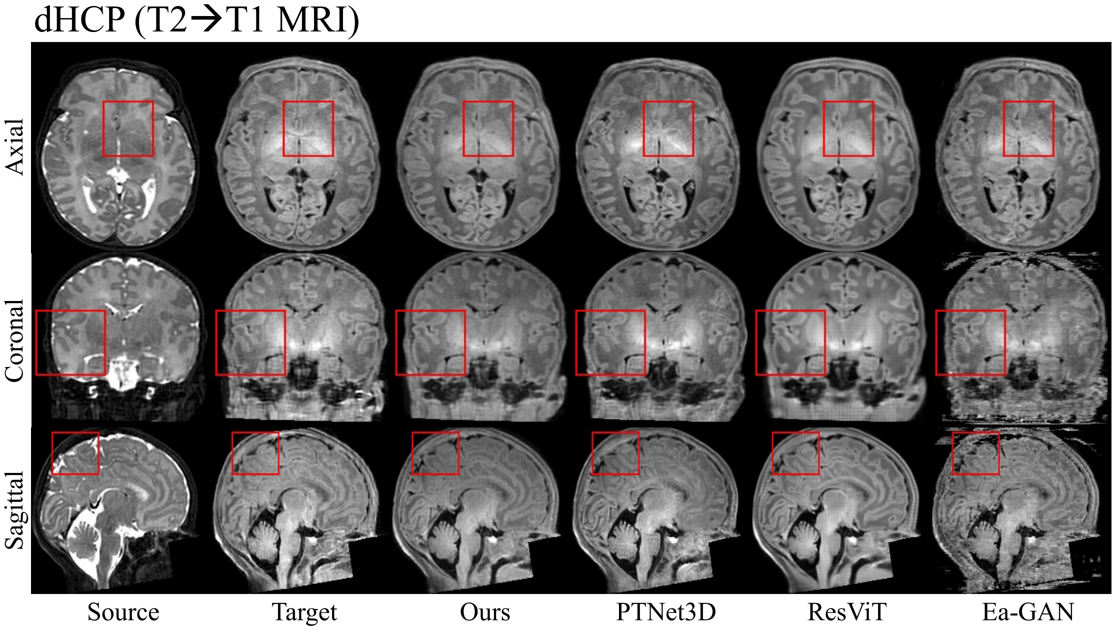
dHCP (T2→T1 MRI)
Axial
Coronal
Sagittal
Source
Target
Ours
PTNet3D
ResViT
Ea-GAN

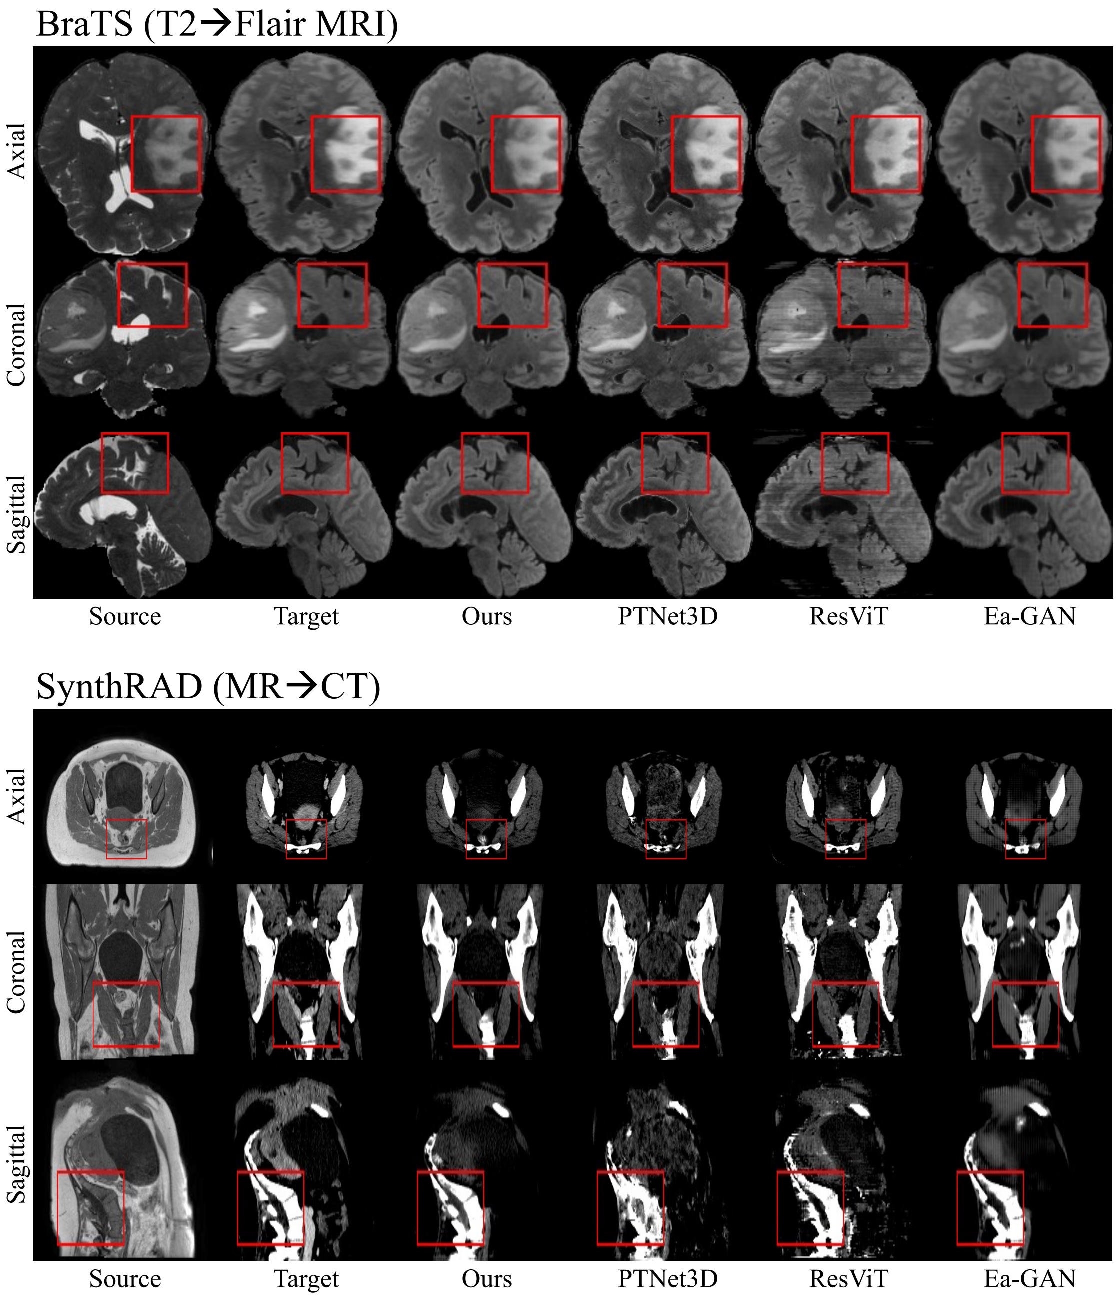
BraTS (T2→Flair MRI)
Axial
Coronal
Sagittal
Source
Target
Ours
PTNet3D
ResViT
Ea-GAN
SynthRAD (MR→CT)
Axial
Coronal
Sagittal
Source
Target
Ours
PTNet3D
ResViT
Ea-GAN

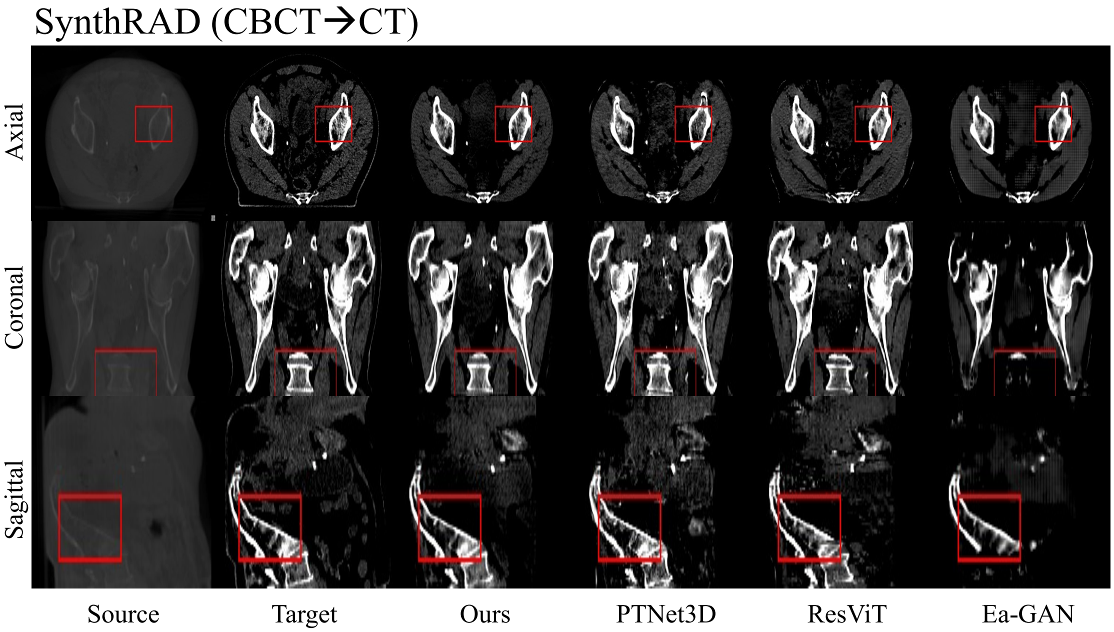

SynthRAD (CBCT→CT)
Axial
Coronal
Sagittal
Source
Target
Ours
PTNet3D
ResViT
Ea-GAN
